# Supplementary material for: Domain dependent Fermi arcs observed in a striped phase dichalcogenide
Source: arXiv:2112.05930 source file (2021-12-11)
Supplement: Supplementary file 1 [file SM_Mizokawa_DomainDepFA.pdf]

# Supplemental Materials on
# Domain dependent Fermi arcs observed in a striped phase dichalcogenide

T. Mizokawa[1], A. Barinov[2], V. Kandyba[2], A. Giampietri[2], R. Matsumoto[1], Y. Okamoto[1], K. Takubo[3], K. Miyamoto[4], T. Okuda[4], S. Pyon[5], H. Ishii[6], K. Kudo[7], M. Nohara[8], and N. L. Saini[9]

[1]Department of Applied Physics, Waseda University, Tokyo 169-8555, Japan. [2]Sincrotrone Trieste S.C.p.A., Area Science Park, 34012 Basovizza, Trieste, Italy. [3]Department of Chemistry, Tokyo Institute of Technology, Meguro, Tokyo 152-8551, Japan. [4]Hiroshima Synchrotron Radiation Center, Hiroshima University, Hiroshima 739-0046, Japan. [5]Department of Applied Physics, The University of Tokyo, Tokyo 113–8656, Japan. [6]Research Institute for Interdisciplinary Science, Okayama University, Okayama 700-8530, Japan. [7]Department of Physics, Osaka University, Toyonaka, Osaka 560-0043, Japan. [8]Department of Quantum Matter, Hiroshima University, Hiroshima 739-8530, Japan.[9]Department of Physics, Universitá di Roma "La Sapienza", 00185 Rome, Italy.

Figures S1(a) and S1(b) show photoemission spectromicroscopy images for the samples quenched quickly to 47 K after cleavage at 300 K and cleaved at 47 K after quenching from 300 K, respectively. The direction of the charge/orbital stripe can be judged from the anisotropy of the Fermi surfaces as shown in Figs. S1(c)-(f). In Fig. S1(a), the major domain with the horizontal charge/orbital stripe has striped texture along its direction. Similar texture is seen in Fig. S1(b) indicating that the striped texture induced by the stress between two phases can survive down to the low temperature in the quenched case while it disappears for slow cooling.

Figure S2(a) shows SARPES spectra of $IrTe_2$ for in-plane spin polarization taken at 20 K with linearly polarized light along the horizontal cut (across the Fermi arc). The $k_x$ positions for Fig. S2(a) are shown in Fig. S2(b) where the spin polarization is plotted as a function of $k_x$ and energy. In addition to the strong spin polarization near $E_F$, spin polarizations with opposite signs are seen around -1.0 eV and -2.0 eV where energy gap is formed due to the spin-orbit interaction between the bulk Te 5p/Ir 5d bands. Therefore, the in-plane spin polarizations of the bulk bands with spin-momentum locking can be assigned to inversion symmetry breaking in the charge-orbital stripe phase although the reported crystal structure keeps it. Another possibility is that surface states are created between the bulk bands from -0.5 eV to -2.5 eV and provide the in-plane spin polarization around -1.0 eV and -2.0 eV. The spin polarization near $E_F$ can be assigned to the quasi one-dimensional surface state in the low temperature phase.

Figure S3(a) shows SARPES spectra of $IrTe_2$ for in-plane spin polarization taken at 20

K with linearly polarized light along the vertical cut (along the Fermi arc). The $k_y$ positions for Fig. S3(a) are shown in Fig. S3(b) where the spin polarization is plotted as a function of $k_y$ and energy. Near the Fermi level, the spin polarization does not change its sign as a fnunction of $k_y$ (along the Fermi arc).

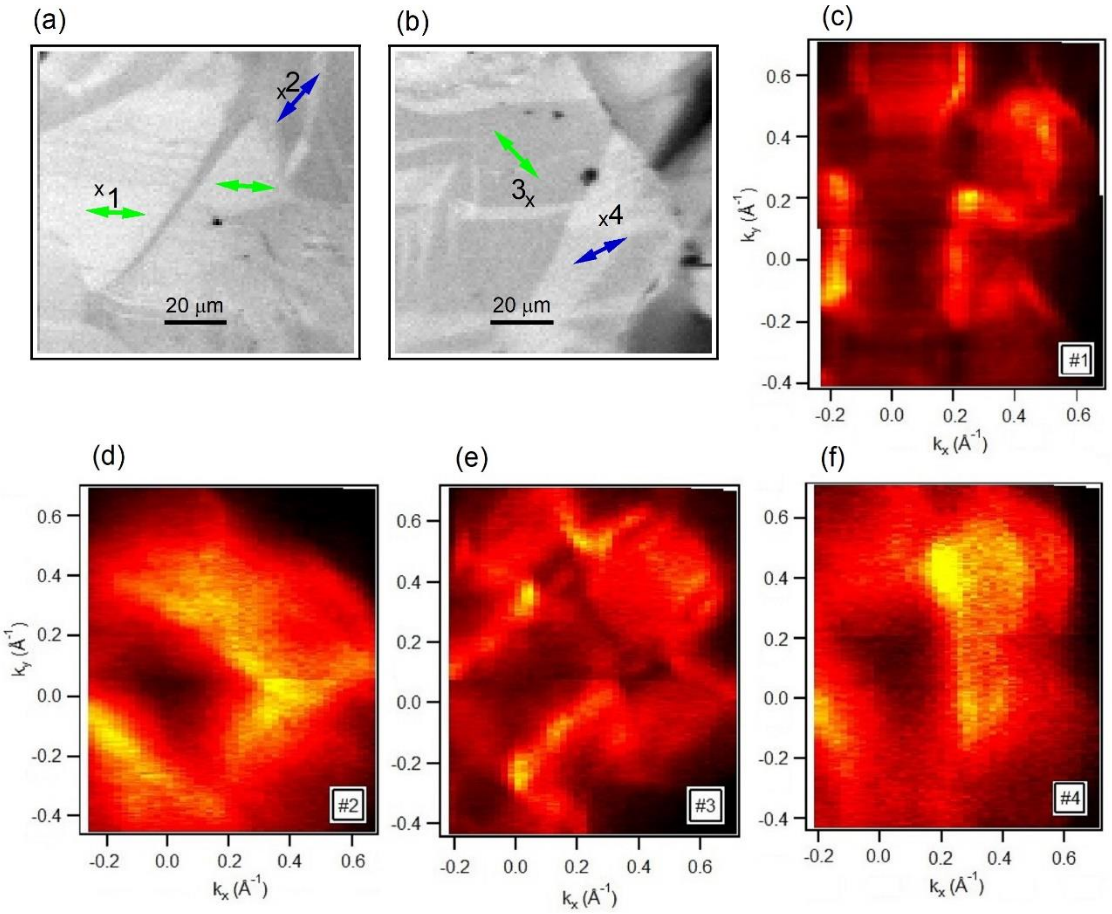


Figure S1: **Domain structure and domain-dependent Fermi surfaces for the quenched IrTe$_2$ single crystal.** (**a**) Domain structure at 47K for the quenched sample after the cleavage. (**b**) Domain structure at 47K for the cleaved sample after the quenching. (**c**) Fermi surfaces for position #1 in (a). Sharp quasi-1D Fermi surfaces are obsered for the majority domain. (**d**) Fermi surfaces for position #2 in (a). Blurred quasi-1D Fermi surfaces are observed for the minority domain. (**e**) Fermi surfaces for position #3 in (b). Sharp quasi-1D Fermi surfaces are observed for the majority domain. (**f**) Fermi surfaces for position #4 in (b). Blurred quasi-1D Fermi surfaces are observed for the minority domain indicating that, while the charge/orbital stripes are well established in the majority domain at the phase transition, they are somewhat disturbed in the minority region for the quenched case.

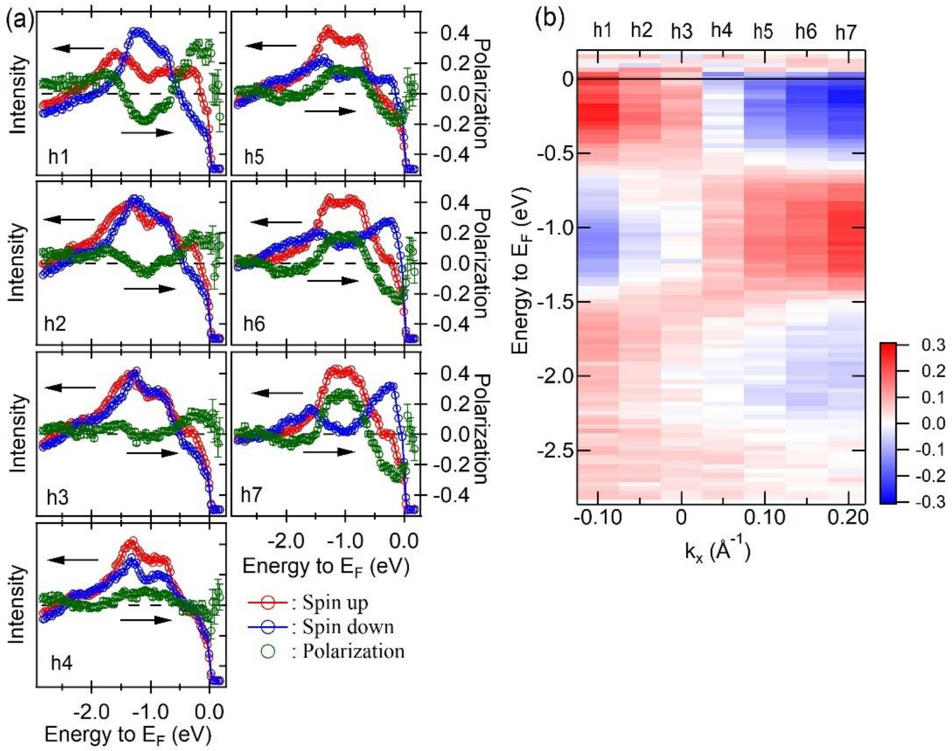


Figure S2: **In-plane spin texture of the bulk and surface bands across the Fermi arc.** (**a**) SARPES spectra of $IrTe_2$ across the Fermi arc taken by linearly polarized hν = 23 eV at 20 K. Spin polarization direction is parallel to the surface. (**b**) Corresponding spin polarization map.

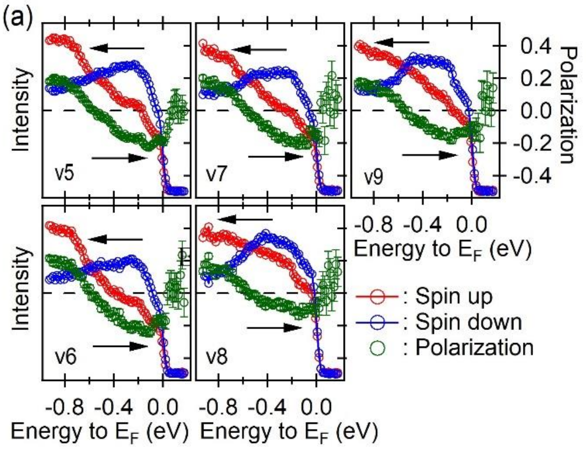


Figure S3: **In-plane spin texture of the bulk and surface bands along the Fermi arc.** (**a**) SARPES spectra of $IrTe_2$ along the Fermi arc taken by linearly polarized hν = 23 eV at 20 K. Spin polarization direction is parallel to the surface. (**b**) Corresponding spin polarization map.
